# Supplementary material for: Understanding first order Raman spectra of boron carbides across the homogeneity range
Source: arXiv:2105.02321 source file (2021-05-05)
Supplement: Supplementary file 1 [file SI_v2.pdf]

# Supplemental material for "Understanding first order Raman spectra of boron carbides across the homogeneity range"

Guido Roma\* and Kevin Gillet

*Université Paris-Saclay, CEA, Service de Recherches de Métallurgie Physique, 91191 Gif sur Yvette, France*

Antoine Jay

*Laboratoire d'analyse et d'architecture des systèmes, CNRS, 31031 Toulouse cedex 4, France*

Nathalie Vast

*Laboratoire des Solides Irradiés, CEA/DRF/IRAMIS, CNRS,  
École Polytechnique, Institut Polytechnique de Paris, 91120 Palaiseau, France*

Gaëlle Gutierrez

*Université Paris-Saclay, CEA, Laboratoire Jannus,  
Service de Recherches de Métallurgie Physique, 91191 Gif sur Yvette, France*

In this supporting information file we provide the following additional information: First, in section A, we report the results on a systematic study of elementary point defects in carbon-rich boron carbide as presented at the International Symposium on Boron, Borides and Related Materials, which took place in Niigata (Japan) in September 2019 (ISBB2019). They are complemented with a few additional graphs and comments and are summarized in Table I of the main paper. In section B we present, in tables and graphical form, the energetics of complex phases of boron carbide defining the convex hull at zero temperature.

Section C discusses the effect of volume relaxation in defect supercells as far as the Raman spectrum is concerned. Section D deals with geometry effects on the Raman spectra of boron carbide supercells containing the “3+1” defect complex. Finally, in section E, we provide Raman maps supporting the identification of grain boundaries in our experimental results.

### **A. Defects formation energies**

The results presented at ISBB2019 as a poster are fully included in the following page. The results have been obtained with the QUANTUM-ESPRESSO package and the same technical details described in the main paper, as far as the exchange-correlation functional (LDA), pseudopotentials, the kinetic energy cutoff,  $\mathbf{k}$ -point sampling and other convergence parameters are concerned.

## Charged defects in B<sub>4</sub>C

Boron carbide is a material supposed to host a variety of point defects or defects complexes. Being a **semiconductor**, point defects can occur in a variety of **charge states**.

Yet no comprehensive *ab initio* study of charged point defects in boron carbide has been done. We present here such a study of **vacancies**, **interstitials** and **antisite** defects, their formation energies and their influence on self-doping.

## Computational details

### Structure B<sub>4</sub>C (20 at% C)

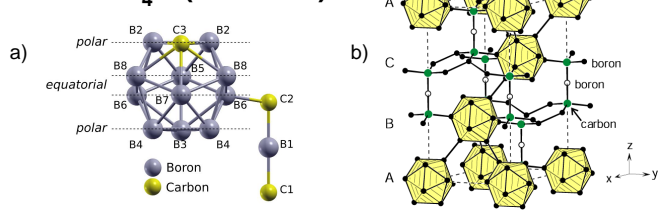

DFT calculations with LDA functional used to compute formation energies as follows:

$$E_f^q(\mu_e) = E_{\text{tot}}^{\text{defect}} - E_{\text{tot}}^{\text{perfect}} + \sum n_i \mu_i + q(\mu_{\text{vbm}} + \mu_e)$$

## Stability of intrinsic defects

**Vacancies** behave mainly as acceptor defects, especially the most stable one, the chain center vacancy which corresponds to a C-C bond<sup>1</sup> in its negative form.

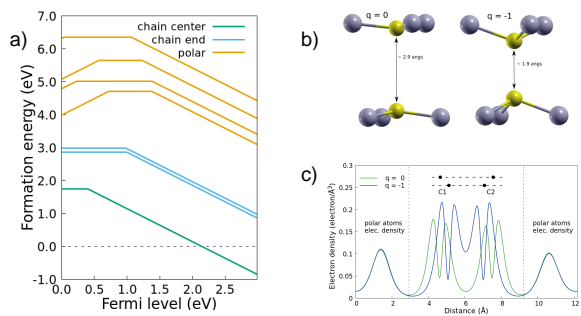

Figure 2: a) formation energies of vacancies, equatorial vacancies are unstable; b) geometric comparison between neutral and negative vacancies; c) electronic density along the defective chain in neutral and negative charge states.

**Antisite's behaviour** depends on its nature, carbon antisites show strong donor behaviour while boron antisites are mostly acceptor defects.

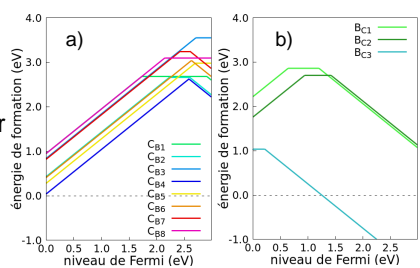

Figure 3: a) formation energies of carbon antisites; b) formation energies of boron antisites.

**Self-interstitial atoms** behave essentially as donor defects, their energy lowers significantly in positive states, reaching 2.3 eV in +3 charge state for boron interstitials

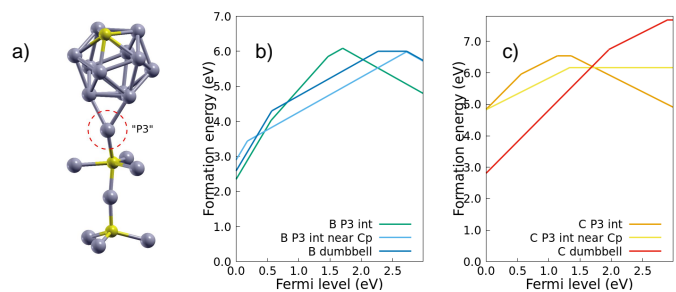

Figure 4: a) so-called P3 boron interstitial; b) formation energies of boron interstitials; c) formation energies of carbon interstitials

## Charge-compensated complexes

Charged defects are associated to form charge-compensated complexes resulting in low-energy defects due to the strong electrostatic interaction.

Bipolar defect<sup>2</sup>: B<sub>10</sub>C<sub>2</sub> + B<sub>12</sub> icosahedra, pair of positive carbon and negative boron antisites.

$$E_f^{\text{B}^{\text{rich}}} = E_f^{\text{C}^{\text{rich}}} = 0.24 \text{ eV}$$

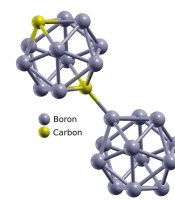

Positive carbon antisite and negative boron vacancy.

$$E_f^{\text{B}^{\text{rich}}} = 2.36 \text{ eV}$$

$$E_f^{\text{C}^{\text{rich}}} = 1.48 \text{ eV}$$

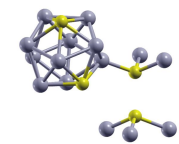

Boron interstitial charged thrice and 3 negative boron antisites.

$$E_f^{\text{B}^{\text{rich}}} = -0.22 \text{ eV}$$

$$E_f^{\text{C}^{\text{rich}}} = 2.11 \text{ eV}$$

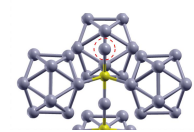

## Conclusions

- Negative chain center vacancy forms C-C bond on the chain.
- Boron interstitial behaviour in B<sub>11</sub>C<sup>p</sup>CBC is in good agreement with its stabilizing effect<sup>3,4</sup> in boron-rich structures: self-interstitials compensate the known electronic deficiency of B<sub>12</sub> icosahedra.
- The association of charged defects in charge compensated complexes leads to new neutral low-energy defects.

## References

- [1] K. Gillet *et al.*, J. Nucl. Mater. **512**, 288 (2018)
- [2] R. Raucoules *et al.*, Phys. Rev. B **84**, 014112 (2011)
- [3] K. Rasim *et al.*, Ang. Chem. Int. Ed. **130**, 6238 (2018)
- [4] A. Jay *et al.*, J. Appl. Phys. **125**, 185902 (2019)

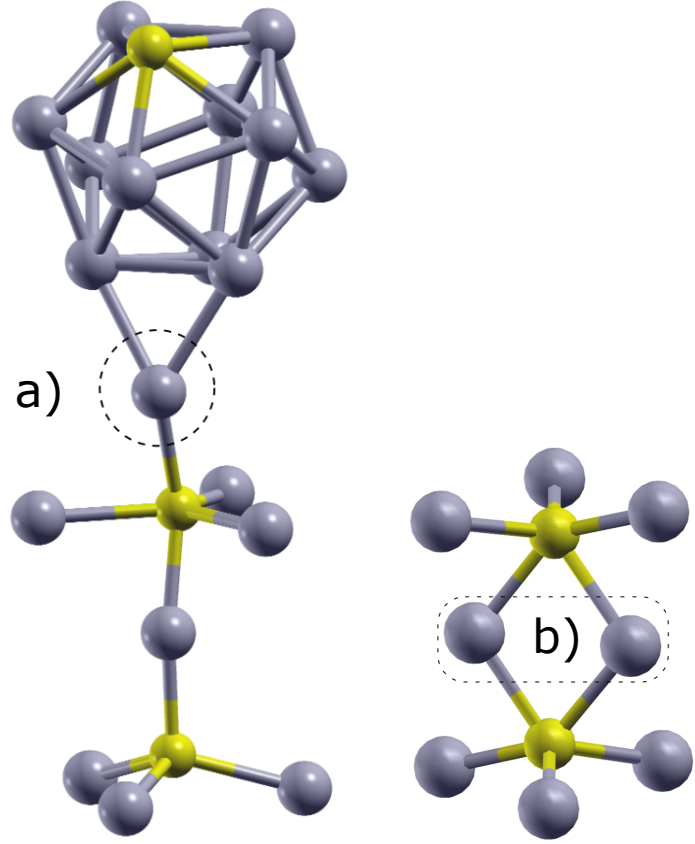

FIG. S1. Two possible structures of boron interstitials in  $(B_{11}C^p)C$ -B-C boron carbide: a) the supplementary boron atom is inserted in the  $2c$  Wyckoff site of the 15-atom rhombohedral structure; b) the  $C\langle\frac{B}{B}\rangle C$  pantograph-like structure obtained when the supplementary boron atom is inserted close to the chain boron atom ( $6g$  Wyckoff site) and relaxed.

We include here as figure S1 the structure of the two boron interstitials considered : the one in figure S1a is the same as that in figure 4a of the attached poster; the second is the pantograph structure named  $C\langle\frac{B}{B}\rangle C$  in the main paper, and which is named B-dumbbell in figure 4b of the poster.

### B. The known convex hull of boron carbide in the homogeneity region

As mentioned in the main manuscript, the “ $(3+1)@27$ ” phase built by inserting a “ $3+1$ ” defect in a  $3\times 3\times 3$   $(B_{11}C)C$ -B-C supercell, is very close to the known convex hull of boron carbide. The data supporting this finding are shown in Table S1, which contains the formation enthalpies of the OPO phases as well as for the “ $(3+1)@27$ ” phase, and two similar ones where the “ $3+1$ ” defects occurs in a different concentration. The results were obtained with a  $\mathbf{k}$ -point sampling

TABLE S1. Formation enthalpy ( $\Delta H_f$ ) large crystal motifs stable OPO phases and stable or metastable (3+1)@ $n$  phases ( $n$  indicates the number of icosahedra in the unit cell).  $\text{OPO}_2^{\text{panto}}$  is a structure where the pantograph variant of the boron interstitial ( $\text{C}(\frac{\text{B}}{\text{B}})\text{C}$  structure) is substituted to interstitials in 2c Wyckoff positions. The standard  $\text{B}_4\text{C}$  phase is shown for comparison. The references are  $\alpha$ -B and graphite.

| Structure                        | $\Delta H_f$ (LDA) | $\Delta H_f$ (optB86b+vdW) | stoichiometry             | C conc. | # of atoms | band gap (LDA) |
|----------------------------------|--------------------|----------------------------|---------------------------|---------|------------|----------------|
|                                  | [eV/atom]          | [eV/atom]                  |                           | at. %   |            | [eV]           |
| ( $\text{B}_{11}\text{C}$ )C-B-C | -0.123             | -0.119                     | $\text{B}_4\text{C}$      | 20      | 15         | 2.99           |
| “(3+1)@64” <sup>a</sup>          | -0.121             | -0.116                     | $\text{B}_{4.1}\text{C}$  | 19.7    | 961        | 2.12           |
| “(3+1)@27”                       | -0.120             | -0.114                     | $\text{B}_{4.2}\text{C}$  | 19.2    | 406        | 2.53           |
| “(3+1)@8”                        | -0.109             | -0.106                     | $\text{B}_{4.8}\text{C}$  | 17.4    | 121        | 1.86           |
| $\text{OPO}_2^{\text{panto}}$    | -0.098             | -0.091                     | $\text{B}_{6.7}\text{C}$  | 13.0    | 414        | 2.19           |
| $\text{OPO}_2$                   | -0.096             | -0.096                     | $\text{B}_{6.7}\text{C}$  | 13.0    | 414        | 2.09           |
| $\text{OPO}_1$                   | -0.070             | -0.073                     | $\text{B}_{10.5}\text{C}$ | 8.7     | 414        | 1.48           |

<sup>a</sup> Computed the  $\Gamma$  point only, corresponding to a  $4\times 4\times 4$   $\mathbf{k}$ -point mesh in the 15-atom unit cell.

TABLE S2. Defect formation energies ( $E_f$ ) of the same structures shown in Table S1 considered as defective structures with respect to the ( $\text{B}_{11}\text{C}$ )C-B-C reference. The standard  $\text{B}_4\text{C}$  phase is shown for comparison. The references are  $\alpha$ -B and graphite. Defect formation energies are given for boron-rich and carbon-rich conditions.

| Structure                     | $E_f^{B-\text{rich}}$ | $E_f^{C-\text{rich}}$ | # of 2c | # of 6g | # of B icos. | # of B chain | $E_f^{C-\text{rich}}/\text{defect}$ | # of atoms/cell |
|-------------------------------|-----------------------|-----------------------|---------|---------|--------------|--------------|-------------------------------------|-----------------|
|                               | [eV]                  | [eV]                  | B EIWS  | B EIWS  | antisites    | antisites    | [eV]                                |                 |
| “(3+1)@64” <sup>a</sup>       | -0.14                 | 2.32                  | 1       | 0       | 3            | 0            | 0.58                                | 961             |
| “(3+1)@27”                    | -0.29                 | 2.18                  | 1       | 0       | 3            | 0            | 0.55                                | 406             |
| “(3+1)@8”                     | -0.23                 | 2.24                  | 1       | 0       | 3            | 0            | 0.56                                | 121             |
| $\text{OPO}_2^{\text{panto}}$ | -6.97                 | 15.19                 | 0       | 9       | 27           | 0            | 0.42                                | 414             |
| $\text{OPO}_2$                | -5.89                 | 16.27                 | 9       | 0       | 27           | 0            | 0.45                                | 414             |
| $\text{OPO}_1$                | -6.57                 | 29.43                 | 9       | 0       | 27           | 18           | 0.55                                | 414             |

<sup>a</sup> Computed with the  $\Gamma$  point only, corresponding to a  $4\times 4\times 4$   $\mathbf{k}$ -point mesh; the result corresponding to a  $8\times 8\times 8$   $\mathbf{k}$ -point grid for  $E_f$  differs by only 0.01 eV.

corresponding to  $6\times 6\times 6$  grid in the 15-atom unit cell, except for the largest cell.

In Table S2 the structures already presented in Table S1 are considered as defective ( $\text{B}_{11}\text{C}$ )C-B-C, which for the OPO structures implies a large number of simple point defects (boron interstitials and antisites). We show the formation energies of such defective structures and the number of simple point defects (boron interstitials and antisites) in which they can be decomposed.

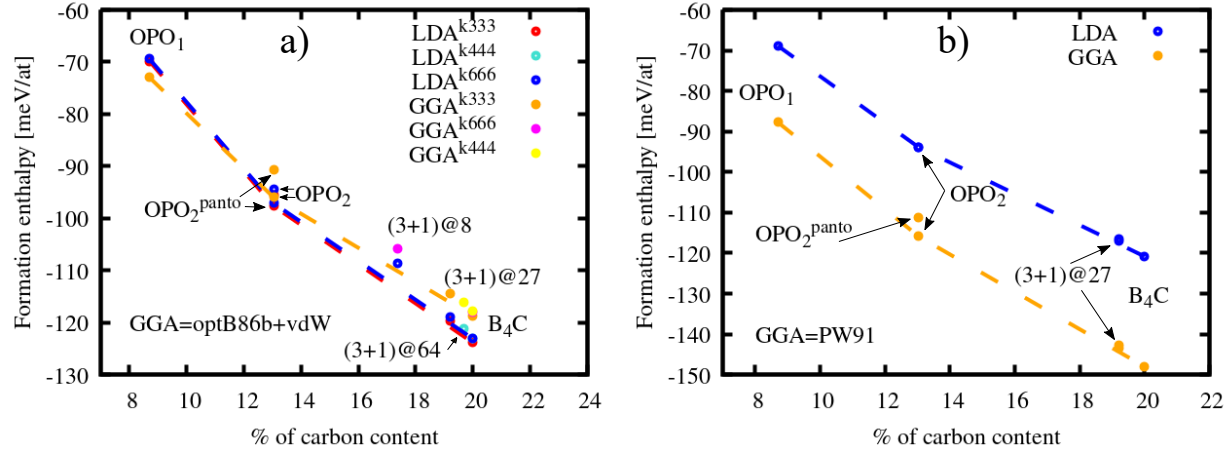

FIG. S2. The convex hull for boron carbide at zero temperature as defined by the OPO structures and the  $(B_{11}C^p)C$ -B-C structure within DFT-LDA and two flavors of DFT-GGA. The GGA results of panel a) were obtained with the optB86b+vdW functional<sup>1</sup>, which contains a long-range correlation term designed to take into account van der Waals interactions. Those of panel b) were obtained with the PW91 GGA functional<sup>4</sup> as in Ref. 5. The LDA pseudopotentials are also different between the two panels.  $3+1^{C=x}$  indicate structures where a “3+1” defect is inserted in a  $B_4C$  supercell at a concentration  $C=x$ . Labels in panel a) indicate the  $\mathbf{k}$ -point sampling of the unit cell ( $kyyy$  refers to sampling of the 15-atom  $B_4C$  unit cell with a  $y \times y \times y$   $\Gamma$ -centered  $\mathbf{k}$ -point grid). Note that within GGA (optB86b+vdW and PW91) the stability of  $OPO_2$  and  $OPO_2^{panto}$  is reversed with respect to LDA. In panel b) the LDA points for  $OPO_2$  and  $OPO_2^{panto}$  are indistinguishable, as well as the  $(3+1)@27$  and its corresponding pantograph variant (not shown in panel a).

Figure S2 shows the convex hull at zero temperature as defined by the OPO structures and the  $(B_{11}C^p)C$ -B-C structure as calculated with the LDA and with two different gradient corrected (GGA) functionals. The structure where we include a “3+1” defect into the  $(B_{11}C^p)C$ -B-C bulk at a defect concentration of 0.25 at. % (or one defect every 27 unit cells) sits practically on this convex hull, as well as for even lower concentration of 0.1 at. % (one 3+1 defect out of 960 atoms). In Fig. S2a the LDA is compared with the optB86b+vdW functional<sup>1</sup>, employed in our previous works on vacancies and helium impurities<sup>2,3</sup>, which contains also a long range correlation term able to correctly describe van der Waals interactions. In Fig S2b we compare to the PW91 GGA functional<sup>4</sup>. Note that within the GGA the order of stability of  $OPO_2$  and  $OPO_2^{panto}$  is reversed:  $OPO_2$  is more stable than  $OPO_2^{panto}$ , while within the LDA the opposite holds.

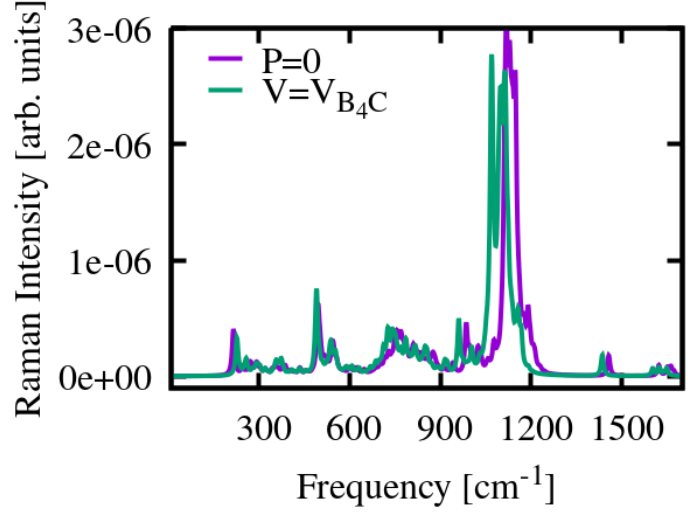

FIG. S3. Comparison of Raman spectra for a  $2 \times 2 \times 2$  supercell of  $B_4C$  containing a boron interstitial ( $2c$  Wyckoff position) in charge state  $3+$  calculated at the relaxed volume of the defected supercell ( $P=0$ ) or at equilibrium volume of undefected  $B_4C$  (the residual pressure is  $-70$  kbar).

### C. Influence of volume relaxation on the Raman spectra of defects

The Raman spectra of defect containing supercells shown in the main paper have been calculated at fixed volume, i.e., at the volume of undefected  $(B_{11}C)C-B-C$ , in order to avoid the arbitrariness of volume relaxation procedures that have been pointed out in the case of charged defects<sup>6</sup>. We wish to show, here, however, that even with volume relaxations, the main characteristics of the Raman spectrum are maintained. We consider here a defect (the boron interstitial in  $2c$  Wyckoff position) with  $+3$  charge state and a relatively large residual pressure negative of  $70$  kbar. The Raman spectrum calculated for the volume relaxed  $2 \times 2 \times 2$  supercell is compared to the fixed volume one in figure S3. The effects amounts mostly in a shift of the peaks, which is more visible in the high frequency part of the spectrum, in particular the intericosahedral modes, the first undergoing the compression<sup>7</sup>. A similar effect was observed for point defects in silicon carbide<sup>8</sup>.

### D. Geometry effects in presence of “3+1” defects/phases

As discussed in the previous subsection and in the main paper, a periodic arrangement of “3+1” defects constitutes a new phase on the convex hull of boron carbide when the concentration coincides with a “3+1” defect in  $27 (B_{11}C)C-B-C$  unit cells. We call this the “(3+1)@27” phase. When the concentration is higher (one “3+1” defect out of  $8 (B_{11}C)C-B-C$  unit cells) the structure lies slightly

above the convex hull. In this subsection we show the effects of light polarization direction with respect to the crystallographic axes on the calculated Raman spectrum of these structures. In Figure S4 we show angular maps similar to those for  $(\text{B}_{11}\text{C})\text{C-B-C}$  shown in Figure 2 of the main paper. The comparison between the two defect concentration is interesting, because while for azimuthal angle  $\theta=30^\circ$  or less (panels a,b,e,f) the difference between the two concentrations is not striking (and similar to the  $\text{B}_4\text{C}$  bulk maps), for  $\theta=60^\circ$  and  $\theta=90^\circ$  the activation of the frequency region between  $\approx 700$  and  $1100 \text{ cm}^{-1}$  is clearly much more pronounced at the higher concentration (panels g,h) than for the lower one (panels c,d).

### E. Experimental identification of grain boundaries

In order to support the identification of grain boundaries in Figure 4a of the main paper, we show here another micrograph of the same region (Fig. S5a); here the grain 1 is in the upper side of the micrograph and grain 2 is in the lower side. The Raman intensity maps corresponding to the region delimited by the white framework are shown for three frequencies:  $480 \text{ cm}^{-1}$  (Fig. S5b),  $970 \text{ cm}^{-1}$  (Fig. S5c), and  $1340 \text{ cm}^{-1}$  (Fig. S5d). The latter frequency is not related to  $\text{B}_4$  Raman spectrum and is probably associated with carbon accumulation in porosities and grain boundaries.

---

\* guido.roma@cea.fr

<sup>1</sup> Klimeš, D. R. Bowler, and A. Michaelides, Phys. Rev. B **83**, 195131 (2011), publisher: American Physical Society.

<sup>2</sup> A. Schneider, G. Roma, J.-P. Crocombette, V. Motte, and D. Gosset, J. Nucl. Mater. **496**, 157 (2017).

<sup>3</sup> K. Gillet, G. Roma, J.-P. Crocombette, and D. Gosset, J. Nucl. Mater. **512**, 288 (2018).

<sup>4</sup> J. P. Perdew and Y. Wang, Phys. Rev. B **45**, 13244 (1992).

<sup>5</sup> A. Jay, O. Hardouin Duparc, J. Sjakste, and N. Vast, Journal of Applied Physics **125**, 185902 (2019), eprint: <https://doi.org/10.1063/1.5091000>.

<sup>6</sup> F. Bruneval, C. Varvenne, J.-P. Crocombette, and E. Clouet, Phys. Rev. B **91**, 024107 (2015).

<sup>7</sup> A. Jay, *Conception in silico d'une nouvelle phase de carbure de bore*, PhD Thesis, École Doctorale Polytechnique (2015).

<sup>8</sup> G. Roma, physica status solidi (a) **213**, 2995 (2016).

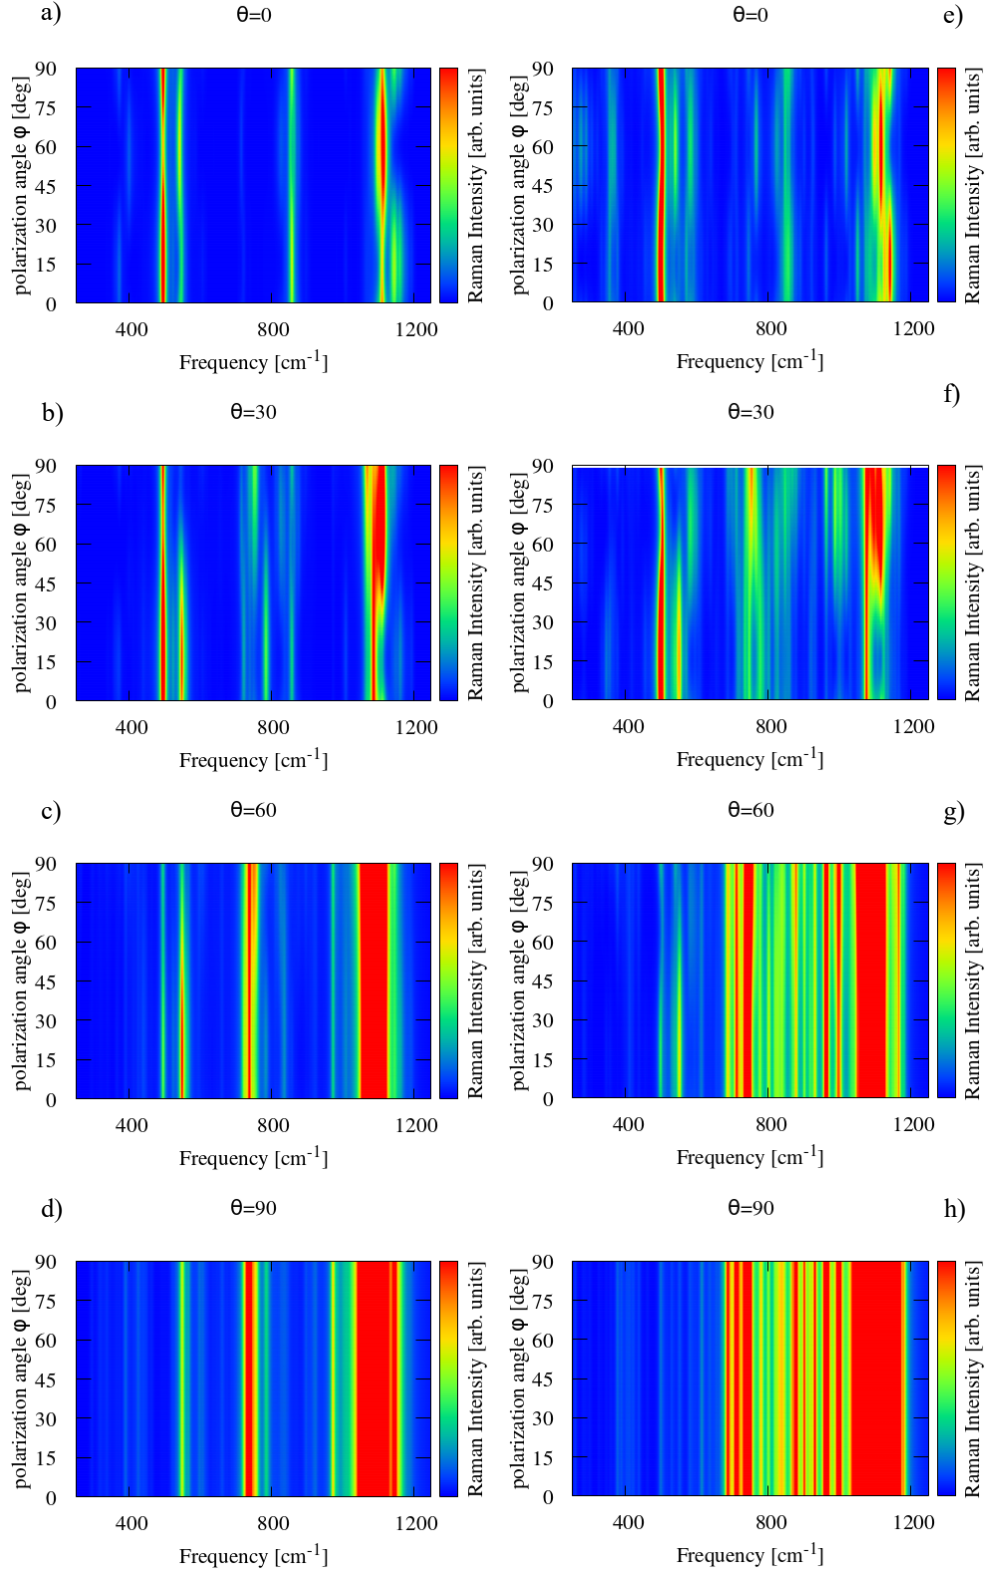

FIG. S4. Maps of the computed Raman intensities vs the polar angle  $\phi$  for four choices of the azimuthal angle  $\theta$ , the angles identifying the geometrical relationship between the propagation directions of the incident and scattered light with respect to the crystal axes. Panels a,b,c,d refer to a  $3 \times 3 \times 3$  supercell of  $\text{B}_4$  containing a "3+1" defect. Panels e,f,g,h refer to a higher concentration of "3+1" defects, one in a  $2 \times 2 \times 2$  supercell of  $\text{B}_4\text{C}$ .

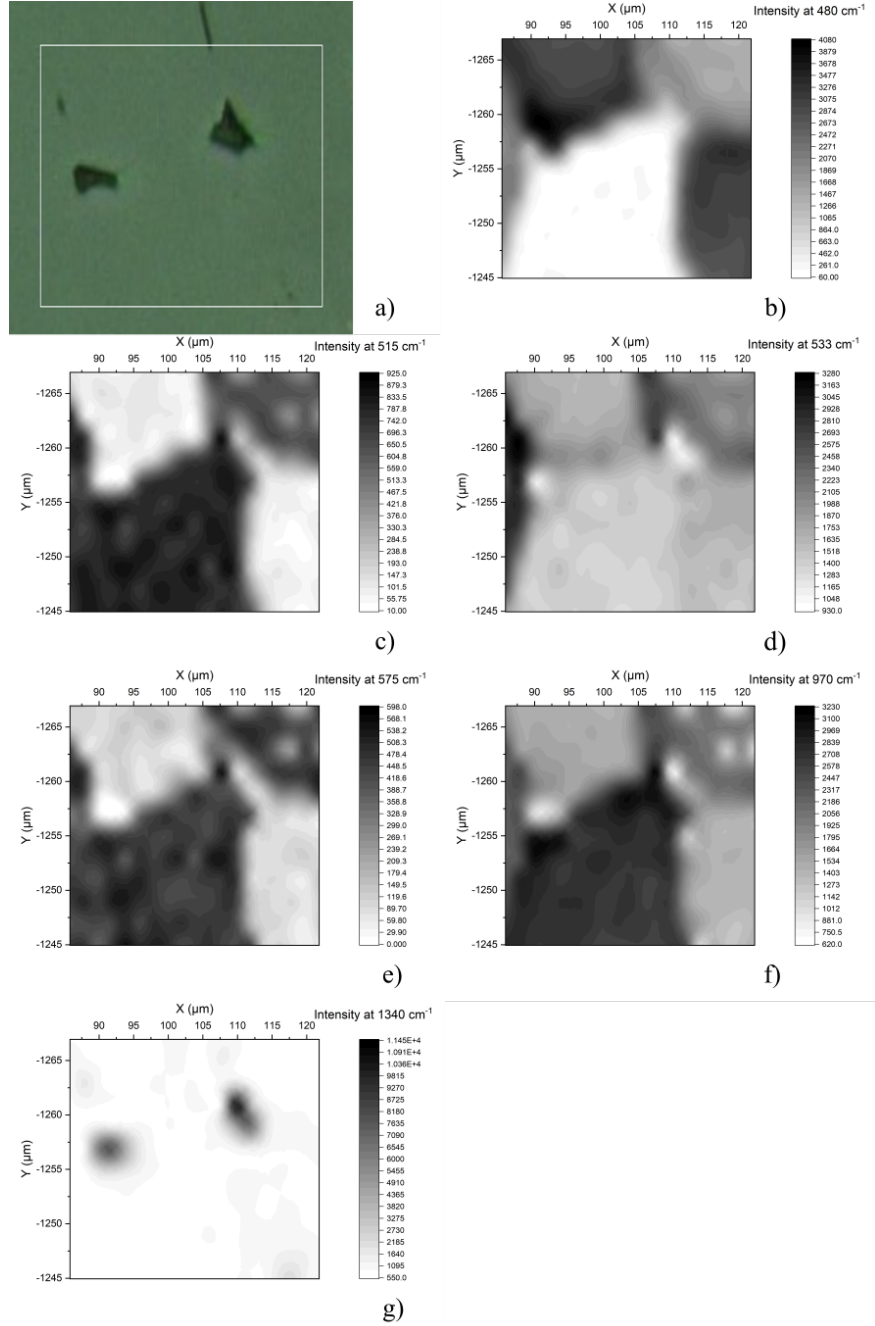

FIG. S5. Raman mapping of a boron carbide sample. Panel a: optical micrograph of the same area shown in Figure 4 of the main paper. The white framework corresponds to the region shown in panels b-g, where spatial maps of the Raman intensities corresponding to frequencies of 480  $\text{cm}^{-1}$  (panel b), 515  $\text{cm}^{-1}$  (panel c), 533  $\text{cm}^{-1}$  (panel d), 575  $\text{cm}^{-1}$  (panel e), 970  $\text{cm}^{-1}$  (panel f), and 1340  $\text{cm}^{-1}$  (panel g) are shown.
